# Supplementary material for: On the surface Bloch waves in truncated periodic media: scalar-wave primer
Source: arXiv:2507.20431 ancillary file (2025-12-02)
Supplement: Supplementary file 1 [file ESM13.pdf]

# Appendix A Properties of the quadratic eigenvalue problem

In this section, we demonstrate various claims made in Section 22.3 concerning the spectral properties of QEP (8). We commence the analysis by introducing an auxiliary mapping $\tilde{\mathcal{A}}: H^1_p(Y) \mapsto H^1_p(Y)$ given by

$$\langle \tilde{\mathcal{A}}\phi, \psi\rangle := \int_Y G\nabla\phi\cdot\nabla\overline{\psi}\,\mathrm{d}Y_{\boldsymbol{x}} - \mathrm{i}\sum_\beta k_\beta\Gamma^{\beta j}\int_Y G\left(\frac{\partial\phi}{\partial x^j}\overline{\psi} - \phi\frac{\partial\overline{\psi}}{\partial x^j}\right)\mathrm{d}Y_{\boldsymbol{x}} + \alpha\int_Y \phi\overline{\psi}\,\mathrm{d}Y_{\boldsymbol{x}}$$

for any $\phi,\psi\in H^1_p(Y)$, where $\alpha$ is a constant sufficiently large so that $\tilde{\mathcal{A}}$ is invertible. To demonstrate the latter property, one can show that $\langle\tilde{\mathcal{A}}\phi,\phi\rangle \geqslant c\|\phi\|_{H^1_p(Y)}$ for some constant $c>0$ by estimating the second term on the right-hand side via Young's inequality $ab\leqslant a^2/(2\epsilon)+\epsilon b^2/2$ for $a,b\geqslant 0$ and suitable $\epsilon>0$.

**Lemma 1.** *Operators $\mathcal{A}: H^1_p(Y)\mapsto H^1_p(Y)$, $\mathcal{B}: H^1_p(Y)\mapsto H^1_p(Y)$ and $\mathcal{C}: H^1_p(Y)\mapsto H^1_p(Y)$ are self-adjoint.*

*Proof.* Since $G$ is real-valued, operator $\mathcal{C}$ is clearly self-adjoint. We next show that $\mathcal{B}$ has the same property. Indeed, for any $\phi,\psi\in H^1_p(Y)$ we have

$$\begin{aligned}\langle\mathcal{B}^*\phi,\psi\rangle &= \langle\phi,\mathcal{B}\psi\rangle = \overline{\langle\mathcal{B}\psi,\phi\rangle} = \overline{2\sum_\beta k_\beta\Gamma^{\alpha\beta}\int_Y G\psi\overline{\phi}\,\mathrm{d}Y_{\boldsymbol{x}} - \mathrm{i}\Gamma^{\alpha j}\int_Y G\left(\frac{\partial\psi}{\partial x^j}\overline{\phi} - \psi\frac{\partial\overline{\phi}}{\partial x^j}\right)\mathrm{d}Y_{\boldsymbol{x}}}\\ &= 2\sum_\beta k_\beta\Gamma^{\alpha\beta}\int_Y G\phi\overline{\psi}\,\mathrm{d}Y_{\boldsymbol{x}} - \mathrm{i}\Gamma^{\alpha j}\int_Y G\left(\frac{\partial\phi}{\partial x^j}\overline{\psi} - \phi\frac{\partial\overline{\psi}}{\partial x^j}\right)\mathrm{d}Y_{\boldsymbol{x}} = \langle\mathcal{B}\phi,\psi\rangle.\end{aligned}$$

The self-adjointness of $\mathcal{A}$ can be demonstrated in an analogous way. □

**Lemma 2.** *Operator $\mathcal{B}: H^1_p(Y)\mapsto H^1_p(Y)$ is compact, and operator*

$$\mathcal{T}(\lambda) = \mathcal{A} + \lambda\mathcal{B} + \lambda^2\mathcal{C}$$

*is Fredholm of index zero.*

*Proof.* We note that $\mathcal{B} = \mathcal{B}_1+\mathcal{B}_2+\mathcal{B}_3$, where

$$\langle\mathcal{B}_1\phi,\psi\rangle = -\mathrm{i}\Gamma^{\alpha j}\int_Y G\frac{\partial\phi}{\partial x^j}\overline{\psi}\,\mathrm{d}Y_{\boldsymbol{x}}, \qquad \langle\mathcal{B}_2\phi,\psi\rangle = \mathrm{i}\Gamma^{\alpha j}\int_Y G\phi\frac{\partial\overline{\psi}}{\partial x^j}\,\mathrm{d}Y_{\boldsymbol{x}}, \quad \forall\phi,\psi\in H^1_p(Y),$$

and

$$\langle\mathcal{B}_3\phi,\psi\rangle = 2\sum_\beta k_\beta\Gamma^{\alpha\beta}\int_Y G\phi\overline{\psi}\,\mathrm{d}Y_{\boldsymbol{x}}, \quad \forall\phi,\psi\in H^1_p(Y).$$

Since $\|\mathcal{B}_2\phi\|_{H^1_p(Y)}\leqslant\|\phi\|_{L^2_p(Y)}$, we find that $\mathcal{B}_2$ is a compact operator due to the compact embedding from $H^1_p(Y)$ into $L^2_p(Y)$. We next interpret $\int_Y G\frac{\partial\phi}{\partial x^j}\overline{\psi}\,\mathrm{d}Y_{\boldsymbol{x}}$ as the duality pairing between $H^{-1}_p(Y)$ and $H^1_p(Y)$ with $L^2_p(Y)$ as the pivoting space, which yields $\|\mathcal{B}_1\phi\|_{H^1_p(Y)}\leqslant\|G\frac{\partial\phi}{\partial x^j}\|_{H^{-1}_p(Y)}$. As a result, $\mathcal{B}_1$ is a compact operator due to compact embedding from $L^2_p(Y)$ into $H^{-1}_p(Y)$. On the other hand, $\mathcal{B}_3$ is a compact operator due to the compact embedding from $H^1_p(Y)$ into $L^2_p(Y)$. It can be demonstrated in a similar way that operators $\mathcal{A}-\tilde{\mathcal{A}}$ and $\mathcal{C}$ are also compact. Lastly, we note that $\mathcal{T}(\lambda)$ is the sum of an invertible operator and a compact operator, whereby operator $\mathcal{T}(\lambda)$ is Fredholm of index zero. □

**Propositon 1.** *If $\mathcal{T}(\lambda)\phi = 0$ for some non-zero $\phi \in H^1_p(Y)$, there must exist a nontrivial $\psi \in H^1_p(Y)$ such that $\mathcal{T}(\bar{\lambda})\psi = 0$. Hence all eigenvalues of QEP (8) come in complex-conjugate pairs.*

*Proof.* Let $\mathcal{T}(\lambda)\phi = 0$ for some nontrivial $\phi \in H^1_p(Y)$, and assume that $\mathcal{T}(\bar{\lambda})\psi \neq 0$ for all non-zero $\psi \in H^1_p(Y)$. Then, since $\mathcal{T}(\bar{\lambda})$ is a Fredholm operator of index zero, $\mathcal{T}(\bar{\lambda})$ is injective and hence invertible. Since $\mathcal{A}$, $\mathcal{B}$ and $\mathcal{C}$ are self-adjoint by Lemma 1, one has that $\mathcal{T}(\bar{\lambda}) = \big(\mathcal{T}(\lambda)\big)^*$ whereby $\big(\mathcal{T}(\lambda)\big)^*$ is also invertible. This is, however, a contradiction since $H^1_p(Y) = \text{Range}\big(\mathcal{T}(\lambda)\big)^* = \big(\text{Null}\mathcal{T}(\lambda)\big)^\perp \neq H^1_p(Y)$. □

**Theorem 1.** *Assume that there exists $\tau \in \mathbb{C}$ such that $\mathcal{T}(\tau)$ is injective. Then the eigenvalues $\lambda$ affiliated with the quadratic pencil $\mathcal{T}(\lambda)$ form a discrete set, with infinity being the only possible accumulation point.*

*Proof.* We first note that $\mathcal{T}(\lambda) = \tilde{\mathcal{A}} + \big(\mathcal{A} - \tilde{\mathcal{A}}\big) + \lambda\mathcal{B} + \lambda^2\mathcal{C}$, where $\tilde{\mathcal{A}}$ is invertible while $\mathcal{A} - \tilde{\mathcal{A}}$, $\mathcal{B}$ and $\mathcal{C}$ are compact. Since by premise there exists $\tau \in \mathbb{C}$ such that $\mathcal{T}(\tau)$ is injective and $\mathcal{T}(\lambda)$ is Fredholm operator of index zero, we conclude that all eigenvalues $\lambda$ form a discrete set with infinity being the only possible accumulation point [**?** , Theorem 12.9]. □

## Appendix B Orthogonal basis for non-bijective undulations

For non-bijective undulations ($P > 1$) featuring "small" supports $\tilde{\Upsilon}_{\mathcal{S}}^{(p)}$ in that $|\tilde{\Upsilon}_{\mathcal{S}}^{(p)}| \ll |\tilde{\Upsilon}_{\mathcal{S}}|$, the Fourier series expansion featured in Sec. 33.3 may itself result in having an ill-conditioned matrix $\boldsymbol{\Psi}(k_e)$ for $k_e$ away from $k_e^\star$, and so jeopardize the analysis. Qualitatively speaking, the problem arises from the fact that the function behavior over very small segments could be reasonably well approximated by *multiple* combinations of Fourier, and so Bloch, terms. To tackle the problem, it is useful to reformulate the matrix eigenvalue problem (34) by resorting to a set of reduced function bases that are orthogonal not only on $\tilde{\Upsilon}_{\mathcal{S}}$, but also on $\tilde{\Upsilon}_{\mathcal{S}}^{(p)}$.

For clarity of discussion, we highlight the approach assuming $d = 2$. Starting from a truncated Fourier basis $\{e^{im\theta}\}_{m=-M}^{M}$ that is orthonormal over $(-\pi, \pi)$, the idea is to seek linear combinations thereof that are also orthogonal over $(-\alpha, \alpha)$ for given $\alpha \in (0, \pi)$. This is accomplished via the introduction of discrete prolate spheroidal wave (DPSW) functions $\chi_m(\theta; \alpha)$ [43] that carry the property

$$\int_{-\alpha}^{\alpha} \chi_m(\theta;\alpha)\,\overline{\chi_n}(\theta;\alpha)\,\mathrm{d}\theta \;=\; \delta_{mn}\,\lambda_m, \qquad m,n = \overline{-M, M} \tag{B.1}$$

where $0 < \lambda_m < 1$ are the eigenvalues of the prolate matrix [43, 47], constructed from $\{e^{im\theta}\}_{m=-M}^{M}$ restricted to $(-\alpha, \alpha)$. Clearly, a DPSW function whose eigenvalue $\lambda_m$ is close to 1 (resp. 0) will have most of its energy localized within $(-\alpha, \alpha)$ (resp. $(-\pi, \pi)\backslash[-\alpha, \alpha]$), see Appendix BAppendix B.1 for details. This result, combined with the property of the prolate matrix that for large $M$ its eigenvalues cluster near 1 and 0, exposes a reduced set of "optimal" basis functions catering for the representation over a symmetric interval $I(\alpha) \subset (-\pi, \pi)$, namely

$$\begin{aligned} &\text{Interior segment } I = (-\alpha,\alpha): && \big\{\chi_m(\theta;\alpha)\colon\, |\lambda_m| > 1-\epsilon\big\} \\ &\text{Exterior segment } I = (-\pi,\pi)\backslash[-\alpha,\alpha]: && \big\{\chi_m(\theta;\alpha)\colon\, |\lambda_m| < \epsilon\big\} \end{aligned}, \tag{B.2}$$

corresponding to a given spectral threshold $\epsilon = o(1)$.

For two-dimensional problems, the unit cell (20) of "in-plane" periodicity $\tilde{\Upsilon}_{\mathcal{S}}$ corresponds to a line segment $(-\tfrac{1}{2}, \tfrac{1}{2})$ spanned by $\zeta := \tilde{x}^\beta$. With reference to Fig. 2 in the manuscript, we can next classify the partial undulation supports $\tilde{\Upsilon}_{\mathcal{S}}^{(p)}$ ($p = \overline{1, P}$) as either *exterior* or *interior* in that

$$\Big(\inf \tilde{\Upsilon}_{\mathcal{S}}^{(p)} = -\tfrac{1}{2} \,\wedge\, \sup \tilde{\Upsilon}_{\mathcal{S}}^{(p)} = \tfrac{1}{2}\Big) = \begin{cases} \bot & \text{for interior } \tilde{\Upsilon}_{\mathcal{S}}^{(p)} \\ \top & \text{for exterior } \tilde{\Upsilon}_{\mathcal{S}}^{(p)} \end{cases}, \tag{B.3}$$

noting that interior segments $\tilde{\Upsilon}_{\mathcal{S}}^{(p)}$ need not themselves be contiguous. In principle, the present analysis can be applied individually to each contiguous part of an interior $\tilde{\Upsilon}_{\mathcal{S}}^{(p)}$; for the sake of brevity, we shall forgo such drill down. With the taxonomy (B.3) in place, one can conveniently introduce the support parameters

$$\big(\alpha_{\inf}^{(p)}, \alpha_{\sup}^{(p)}\big) := \begin{cases} 2\pi\Big(\inf \tilde{\Upsilon}_{\mathcal{S}}^{(p)}, \sup \tilde{\Upsilon}_{\mathcal{S}}^{(p)}\Big) & \text{for interior } \tilde{\Upsilon}_{\mathcal{S}}^{(p)} \\ 2\pi\Big(\inf \tilde{\Upsilon}_{\mathcal{S}}\backslash\tilde{\Upsilon}_{\mathcal{S}}^{(p)}, \sup \tilde{\Upsilon}_{\mathcal{S}}\backslash\tilde{\Upsilon}_{\mathcal{S}}^{(p)}\Big) & \text{for exterior } \tilde{\Upsilon}_{\mathcal{S}}^{(p)} \end{cases}, \tag{B.4}$$

which enable the generation of a reduced orthogonal basis over each $\tilde{\Upsilon}_{\mathcal{S}}^{(p)}$ ($p = \overline{1, P}$) by letting

$$\theta \mapsto \theta^{(p)}(\zeta) := 2\pi\zeta - \tfrac{1}{2}\big(\alpha_{\sup}^{(p)} + \alpha_{\inf}^{(p)}\big), \qquad \alpha \mapsto \alpha^{(p)} := \tfrac{1}{2}\big(\alpha_{\sup}^{(p)} - \alpha_{\inf}^{(p)}\big). \tag{B.5}$$

In the sequel, we refer to the reduced bases due to (B.2)–(B.5) by

$$\big\{\hat{\chi}_q^{(p)}(\zeta) := \chi_{m_q}(\theta^{(p)}; \alpha^{(p)})\big\}_{q=1}^{Q_p}, \qquad m_q \in \{-M, -M+1, \ldots, M\},$$

where $Q_p$ is the size of the reduced basis over $\tilde{\Upsilon}_S^{(p)}$ stemming from (B.2). This allows us to recast the Fourier series expansion (32) in terms of the reduced basis as

$$\begin{aligned} H^{(p)}(\zeta) \sum_{n=1}^{N} a_n \, \hat{\tau}_n^{(p)}(\zeta) &= \sum_{q=1}^{Q_p} \left\{ \sum_{n=1}^{N} a_n \hat{\psi}_{qn}^{(p)} \right\} \hat{\chi}_q^{(p)}(\zeta), \\ \hat{\psi}_{qn}^{(p)} &= \big(\lambda_q^{(p)}\big)^{-\frac{1}{2}} \int_{-\frac{1}{2}}^{\frac{1}{2}} H^{(p)}(\zeta) \, \hat{\tau}_n^{(p)}(\zeta) \, \overline{\hat{\chi}_q^{(p)}}(\zeta) \, \mathrm{d}\zeta, \qquad p = \overline{1, P} \end{aligned} \tag{B.6}$$

where $\lambda_q^{(p)}$ are the eigenvalues of the prolate matrix $\boldsymbol{P}(\alpha^{(p)})$ corresponding to $\hat{\chi}_q^{(p)}$. By virtue of (B.6), Fourier series-based boundary condition (33) can be rewritten in a reduced form as

$$\sum_{n=1}^{N} \hat{\psi}_{qn}^{(p)} \, a_n = 0 \quad \text{for} \quad q = \overline{1, Q_p} \;\; \text{and} \;\; p = \overline{1, P}, \tag{B.7}$$

resulting in a surface-wave eigenproblem of form (34), where $\boldsymbol{\Psi} = \boldsymbol{\Psi}(k_e)$ is a complex-valued $(\sum_{p=1}^{P} Q_p) \times N$ matrix collecting $\hat{\psi}_{qn}^{(p)}$; $k_e$ is a prescribed wavenumber in direction $\boldsymbol{e}$ featured by the QEP (15), and $\boldsymbol{a} = \boldsymbol{a}(k_e) \in \mathbb{C}^N$ is the vector of Bloch wave amplitudes $a_n$. Clearly, the first dimension of $\boldsymbol{\Psi}$ is now reduced relative to that stemming from the Fourier series expansion since

$$Q_p < 2M+1 \quad \Longrightarrow \quad \sum_{p=1}^{P} Q_p < P(2M+1).$$

By analogy to (35), we require that

$$\sum_{p=1}^{P} Q_p \geqslant N$$

which ensures that the number of data is not exceeded by the number of unknowns, $N$.

## Appendix B.1 Discrete prolate spheroidal wave functions

For clarity of discussion, we shall temporarily work with vectors and and matrices whose components carry sign-indefinite indexes. Specifically, for $M \in \mathbb{Z}^+$ we let

$$\boldsymbol{b} := \big(b_m\big), \qquad \boldsymbol{A} := \big(A_{mn}\big), \qquad m, n = \overline{-M, M}$$

denote a $(2M+1)$ vector and a $(2M+1) \times (2M+1)$ matrix, respectively. On letting

$$\varphi_m(\theta) := \frac{1}{\sqrt{2\pi}} e^{im\theta}, \quad m = 0, \pm 1, \pm 2, \cdots \tag{B.8}$$

which form a complete orthonormal basis in $L^2(-\pi, \pi)$, for fixed $\alpha \in (0, \pi]$ we first introduce a $(2M+1) \times (2M+1)$ matrix function $\boldsymbol{P}(\alpha)$ with entries

$$P_{mn} := \int_{-\alpha}^{\alpha} \varphi_m(\theta) \, \overline{\varphi_n(\theta)} \, \mathrm{d}\theta = \frac{1}{2\pi} \int_{-\alpha}^{\alpha} e^{i(m-n)\theta} \, \mathrm{d}\theta = \begin{cases} \frac{\alpha}{\pi}, & m = n \\ \frac{\sin((m-n)\alpha)}{\pi(m-n)}, & m \neq n \end{cases}, \quad m, n = \overline{-M, M}. \tag{B.9}$$

One may observe that $\boldsymbol{P}(\alpha)$ is the well-known prolate matrix which frequently appears in signal processing. In the following lemma, we collect several useful properties [43, 47] of the prolate matrix.

**Lemma 3.** *Let $\boldsymbol{P}(\alpha)$ be the $(2M+1)\times(2M+1)$ prolate matrix for given $\alpha \in (0,\pi)$, and let $\{\lambda_m(\alpha)\}$ denote its eigenvalues arranged in a descending order.*

- $1 > \lambda_{-M} > \lambda_{-M+1} > \cdots > \lambda_M > 0$;
- *For large $M$, the eigenvalues $\{\lambda_m\}$ cluster near 1 and 0. More specifically, letting $N_e(a,b)$ denote the number of eigenvalues contained within the interval $[a,b] \subseteq (0,1]$ it can be shown that*
  - *for any $0 < a < b < 1$, $\lim_{M\to\infty} \frac{N_e(a,b)}{2M+1} = 0$, i.e. the eigenvalues $\{\lambda_m(\alpha)\}$ cluster near 1 and 0;*
  - *for any $0 < a < b = 1$, $\lim_{M\to\infty} \frac{N_e(a,b)}{2M+1} = \frac{\alpha}{\pi}$, i.e. the number of eigenvalues $\{\lambda_m(\alpha)\}$ clustered near 1 (resp. 0) scales with $\alpha/\pi$ (resp. $1-\alpha/\pi$);*
- *The eigenvalues satisfy the "symmetry" relationship*

$$\lambda_m(\alpha) + \lambda_{-m}(\pi - \alpha) = 1, \quad m = \overline{-M, M};$$

- *$\boldsymbol{P}(\pi)$ is the identity matrix; As $\alpha \to 0$, $\boldsymbol{P}(\alpha)$ becomes ill-conditioned due to the fact that*

$$\lim_{\alpha\to 0} P_{mn} = \frac{\alpha}{\pi}, \qquad m,n = \overline{-M, M}.$$

On recalling the singular value decomposition of $\boldsymbol{P}(\alpha)$ given by

$$\boldsymbol{P}(\alpha) = \boldsymbol{U}\boldsymbol{\Sigma}\boldsymbol{U}^{\mathrm{T}} \tag{B.10}$$

where $\boldsymbol{U}$ is an orthogonal matrix with components $U_{mn} = U_{mn}(\alpha)$ and

$$\boldsymbol{\Sigma} = \mathrm{diag}(\lambda_{-M}, \lambda_{-M+1}, \cdots, \lambda_M),$$

we are now in position to introduce the Slepian's discrete prolate spheroidal wave (DPSW) functions given by

$$\chi_m(\theta;\alpha) := \sum_{n=-M}^{M} U_{nm}(\alpha)\,\varphi_n(\theta), \qquad m = \overline{-M, M} \tag{B.11}$$

It is known that (B.11) are *doubly orthogonal*, see for instance [43]. Specifically, one finds from (B.8)–(B.11) that $\chi_m$ satisfy

$$\begin{aligned} \int_{-\pi}^{\pi} \chi_m(\theta;\alpha)\,\overline{\chi_n}(\theta;\alpha)\,\mathrm{d}\theta &= \delta_{mn}, \\ \int_{-\alpha}^{\alpha} \chi_m(\theta;\alpha)\,\overline{\chi_n}(\theta;\alpha)\,\mathrm{d}\theta &= \delta_{mn}\,\lambda_m, \qquad m,n = \overline{-M, M} \end{aligned} \tag{B.12}$$

where $\delta_{mn}$ is the Kronecker delta. The fact that for large $M$ the eigenvalues $\lambda_m(\alpha)$ cluster near either 1 or 0 implies that, when $\lambda_m$ is close to 1, the "principal energy" of a DPSW function $\chi_m$ is localized within the segment $(-\alpha,\alpha)$. Conversely when $\lambda_m$ is close to 0, the "principal energy" of $\chi_m$ is (for large $M$) confined to the interval $(-\pi,\pi)\backslash[-\alpha,\alpha]$.

To obtain an optimal reduced basis over a symmetric line segment $I \subset (-\pi,\pi)$ controlled by $\alpha$, we accordingly focus on $\lambda_m$ whose respective DPSW functions $\chi_m$ have a meaningful portion of their energy contained within $I$. For a given spectral cutoff $\epsilon$, this leads to a reduced set of basis functions

$$\begin{array}{rl} \text{Interior segment, } I = (-\alpha,\alpha): & \{\chi_m(\theta;\alpha) \colon |\lambda_m| > 1-\epsilon\} \\ \text{Exterior segment, } I = (-\pi,\pi)\backslash[-\alpha,\alpha]: & \{\chi_m(\theta;\alpha) \colon |\lambda_m| < \epsilon\} \end{array}, \qquad \epsilon = o(1). \tag{B.13}$$

Recalling Lemma 3 we observe that as $M \to \infty$, the size of a reduced basis over an interior segment scales with $\alpha/\pi$. This results in having only a few basis functions $\chi_m$ due to (B.13) when considering either "short" *interior* segments (i.e. small $\alpha$), or "short" *exterior* segments (i.e. small $\pi - \alpha$).

## Appendix C Corroborating estimates

In support of the claims made in Section 33.4, we next establish the key estimates describing the "high-wavenumber" behavior of quadratic eigenfunctions $\tilde{\phi}_n$ solving (15) when $|\tilde{\kappa}_n| \gg |k_e|$. For clarity, we start with a simple example (two-dimensional orthogonal lattice, surface cut parallel to a lattice basis vector), and then proceed to the general case governed by QEP (15).

### Appendix C.1 Orthogonal Bravais lattice, $d = 2$.

Assuming an orthogonal Bravais lattice $\boldsymbol{R} \subset \mathbb{R}^2$ in a Cartesian frame endowed with an orthonormal basis $(\boldsymbol{e}_1, \boldsymbol{e}_2)$ and letting $\boldsymbol{e} = \boldsymbol{e}_1$ reduces QEP (15) to (9), which we examine first.

**Proof of eq. (47).**

*Proof.* Letting $\psi = \phi_n$ in (9), we obtain

$$-\kappa_n^2 \int_Y G\phi_n\overline{\phi_n}\,\mathrm{d}Y_{\boldsymbol{\xi}} \;=\; 2\kappa_n \int_Y G\,\Im\left[\frac{\partial\phi_n}{\partial\xi_2}\overline{\phi_n}\right]\mathrm{d}Y_{\boldsymbol{\xi}} + 2k_1\int_Y G\,\Im\left[\frac{\partial\phi_n}{\partial\xi_1}\overline{\phi_n}\right]\mathrm{d}Y_{\boldsymbol{\xi}} + \int_Y G\nabla\phi_n\cdot\nabla\overline{\phi_n}\,\mathrm{d}Y_{\boldsymbol{\xi}} + \int_Y (k_1^2G-\omega^2\rho)\,\phi_n\overline{\phi_n}\,\mathrm{d}Y_{\boldsymbol{\xi}}, \tag{C.1}$$

recalling that $\|\phi_n\|_{L^2_p(Y)} = 1$ by premise. To investigate the asymptotic behavior of (C.1) for large $|\kappa_n|$, we introduce the scaling parameter

$$\epsilon \;=\; \epsilon(n) \;:=\; \frac{|k_1|}{|\kappa_n|} \;=\; o(1). \tag{C.2}$$

Letting

$$\boldsymbol{k} \;=\; \kappa_n\,\boldsymbol{v}, \qquad \boldsymbol{v} := \epsilon\, e^{\mathrm{i}\varphi_n}\,\boldsymbol{e}_1 + \boldsymbol{e}_2, \qquad \varphi_n \;=\; \arg\left(\frac{k_1}{\kappa_n}\right)$$

where $(\boldsymbol{e}_1, \boldsymbol{e}_2)$ is the reference orthonormal basis, this allows us to recast (C.1) as

$$-\kappa_n^2 \int_Y G\phi_n\overline{\phi_n}\,\mathrm{d}Y_{\boldsymbol{\xi}} \;=\; 2\kappa_n \int_Y G\boldsymbol{v}\cdot\Im\left[\nabla\phi_n\,\overline{\phi_n}\right]\mathrm{d}Y_{\boldsymbol{\xi}} + \int_Y G\nabla\phi_n\cdot\nabla\overline{\phi_n}\,\mathrm{d}Y_{\boldsymbol{\xi}} + \int_Y (k_1^2G-\omega^2\rho)\,\phi_n\overline{\phi_n}\,\mathrm{d}Y_{\boldsymbol{\xi}}. \tag{C.3}$$

By the triangle inequality and Cauchy–Schwarz inequality, we obtain

$$\begin{aligned}
\left|\int_Y G\boldsymbol{v}\cdot\Im\left[\nabla\phi_n\,\overline{\phi_n}\right]\mathrm{d}Y_{\boldsymbol{\xi}}\right| &\leqslant G_{\sup}\left|\int_Y \boldsymbol{v}\cdot\Im\left[\nabla\phi_n\,\overline{\phi_n}\right]\mathrm{d}Y_{\boldsymbol{\xi}}\right| \\
&\leqslant G_{\sup}\left\{\epsilon\left|\int_Y \Im\left[\frac{\partial\phi_n}{\partial\xi_1}\overline{\phi_n}\right]\mathrm{d}Y_{\boldsymbol{\xi}}\right| + \left|\int_Y \Im\left[\frac{\partial\phi_n}{\partial\xi_2}\overline{\phi_n}\right]\mathrm{d}Y_{\boldsymbol{\xi}}\right|\right\} \\
&\leqslant G_{\sup}(1+\epsilon)\sum_j\left|\int_Y \Im\left[\frac{\partial\phi_n}{\partial\xi_j}\overline{\phi_n}\right]\mathrm{d}Y_{\boldsymbol{\xi}}\right| \\
&\leqslant G_{\sup}(1+\epsilon)\sum_j\left|\int_Y \left|\frac{\partial\phi_n}{\partial\xi_j}\overline{\phi_n}\right|\mathrm{d}Y_{\boldsymbol{\xi}}\right| \\
&\leqslant G_{\sup}(1+\epsilon)\sum_j\left\|\frac{\partial\phi_n}{\partial\xi_j}\right\|_{L^2_p(Y)} \\
&\leqslant \sqrt{2}\,G_{\sup}(1+\epsilon)\,\|\nabla\phi_n\|_{L^2_p(Y)} \;<\; 2\sqrt{2}\,G_{\sup}\,\|\nabla\phi_n\|_{L^2_p(Y)}
\end{aligned} \tag{C.4}$$

for $\epsilon < 1$. Using (C.4) and the triangle inequality applied to the right-hand side of (C.3), we obtain

$$4\sqrt{2}\,|k_1|\,\frac{1}{\epsilon}\,G_{\sup}\,\|\nabla\phi_n\|_{L^2_p(Y)} \,+\, G_{\sup}\,\|\nabla\phi_n\|^2_{L^2_p(Y)} \,+\, (|k_1|^2 G_{\sup} + \omega^2\rho_{\sup}) \\ \geqslant\; |k_1|^2\,\frac{1}{\epsilon^2}\int_Y G\,|\phi_n|^2\,\mathrm{d}Y_{\boldsymbol{\xi}} \;\geqslant\; |k_1|^2\,\frac{1}{\epsilon^2}\,G_{\inf}, \tag{C.5}$$

which can be conveniently restated as

$$\epsilon\left(4\sqrt{2}\,|k_1|\,\|\nabla\phi_n\|_{L^2_p(Y)}\right) + \epsilon^2\,\|\nabla\phi_n\|^2_{L^2_p(Y)} \;\geqslant\; \frac{|k_1|^2}{G_{\sup}}\left(G_{\inf} - \epsilon^2\Big(G_{\sup} + \frac{\omega^2\rho_{\sup}}{|k_1|^2}\Big)\right). \tag{C.6}$$

Letting

$$\alpha \;:=\; \epsilon\,\|\nabla\phi_n\|_{L^2_p(Y)}, \tag{C.7}$$

(C.6) yields the inequality

$$4\sqrt{2}|k_1|\alpha \,+\, \alpha^2 \;>\; \gamma\,|k_1|^2, \qquad \gamma \;=\; \frac{1}{G_{\sup}}\left(G_{\inf} - \epsilon^2\Big(G_{\sup} + \frac{\omega^2\rho_{\sup}}{|k_1|^2}\Big)\right) \;>\; c'\,\frac{G_{\inf}}{G_{\sup}} \tag{C.8}$$

for sufficiently small $\epsilon$ and some $0 < c' < 1$ (close to unity) independent of $\epsilon$. As a result, we obtain

$$\alpha \;>\; c\,|k_1|, \qquad\qquad c \;=\; \sqrt{8+\gamma} - 2\sqrt{2} \;>\; 0, \tag{C.9}$$

for sufficiently small $\epsilon$ and $\gamma \simeq G_{\inf}/G_{\sup}$. By virtue of (C.7) and (C.9), we find that for sufficiently small $\epsilon$ the norm of the gradient is bounded from below by

$$\|\nabla\phi_n\|_{L^2_p(Y)} \;>\; c\,|\kappa_n|, \qquad 0 \;<\; c \;\simeq\; \left(8 + \frac{G_{\inf}}{G_{\sup}}\right)^{\frac{1}{2}} - 2\sqrt{2}. \tag{C.10}$$

□

**Justification of eq. (48).**

In light of (C.10), it is next of interest to examine the QEP-driven anisotropy of

$$\|\nabla\phi_n\|^2_{L^2_p(Y)} \;=\; \left\|\frac{\partial\phi_n}{\partial\xi_1}\right\|^2_{L^2_p(Y)} + \left\|\frac{\partial\phi_n}{\partial\xi_2}\right\|^2_{L^2_p(Y)} \tag{C.11}$$

for $\epsilon \ll 1$ i.e. $|\kappa_n| \gg |k_1|$, manifest in the respective scalings with $\epsilon$ of the summands in (C.11). To this end, we consider an infinitesimal change

$$\omega \;\mapsto\; \omega + \delta\omega$$

of the input frequency in QEP (9), which causes the eigenspectrum perturbations

$$\kappa_n \;\mapsto\; \kappa_n + \delta\kappa_n, \qquad \phi_n \;\mapsto\; \phi_n + \delta\phi_n, \qquad \nabla\phi_n \;\mapsto\; \nabla\phi_n + \delta\nabla\phi_n. \tag{C.12}$$

Focusing on the components of $\delta\nabla\phi_n$, from the linearized statement of $\delta(9)$ we find that

$$2\kappa_n\delta\kappa_n\int_Y G\phi_n\overline{\psi}\,\mathrm{d}Y_{\boldsymbol{\xi}} + (\kappa_n^2+\kappa_1^2)\int_Y G\delta\phi_n\overline{\psi}\,\mathrm{d}Y_{\boldsymbol{\xi}} \,-\, \mathrm{i}\delta\kappa_n\int_Y G\left(\frac{\partial\phi_n}{\partial\xi_2}\overline{\psi} - \phi_n\frac{\partial\overline{\psi}}{\partial\xi_2}\right)\mathrm{d}Y_{\boldsymbol{\xi}} \\ -\,\mathrm{i}\kappa_n\int_Y G\left(\delta\left(\frac{\partial\phi_n}{\partial\xi_2}\right)\overline{\psi} - \delta\phi_n\frac{\partial\overline{\psi}}{\partial\xi_2}\right)\mathrm{d}Y_{\boldsymbol{\xi}} \,-\, \mathrm{i}k_1\int_Y G\left(\delta\left(\frac{\partial\phi_n}{\partial\xi_1}\right)\overline{\psi} - \delta\phi_n\frac{\partial\overline{\psi}}{\partial\xi_1}\right)\mathrm{d}Y_{\boldsymbol{\xi}} \\ +\int_Y\left(G\delta\nabla\phi_n\cdot\nabla\overline{\psi} \,-\, \omega^2\rho\,\delta\phi_n\overline{\psi} - 2\omega\,\delta\omega\,\rho\,\phi_n\overline{\psi}\right)\mathrm{d}Y_{\boldsymbol{\xi}} \;=\; 0 \qquad \forall\psi\in H^1_p(Y), \tag{C.13}$$

where $\|\phi_n\|_{L^2_p(Y)} = 1$ and $\|\nabla\phi_n\|_{L^2_p(Y)} > c|\kappa_n|$ due to (C.10). In light of (C.13), we first consider the "default" isotropic scaling

$$\left\|\delta\Big(\frac{\partial\phi_n}{\partial\xi_2}\Big)\right\|_{L^2_p(Y)} = O\left(\left\|\delta\Big(\frac{\partial\phi_n}{\partial\xi_1}\Big)\right\|_{L^2_p(Y)}\right) = O\big(\|\delta\nabla\phi_n\|_{L^2_p(Y)}\big)$$

of the components of $\delta\nabla\phi_n$. By the arbitrariness of the unperturbed state $(\omega,k_1)$, this hypothesis implies (via integration with respect to $\omega$ starting from $\omega=0$) that

$$\|\boldsymbol{e}_2\cdot\nabla\phi_n\|_{L^2_p(Y)} = O\big(\|\boldsymbol{e}_1\cdot\nabla\phi_n\|_{L^2_p(Y)}\big) = O\big(\epsilon\,\|\nabla\phi_n\|_{L^2_p(Y)}\big).$$

For $|\kappa_n| \gg |k_1|$, this assumption would eliminate the terms containing $k_1$ from the leading-behavior of (C.13) and so *suppress the sensitivity* of quadratic eigenmode perturbations to $k_1$. This is a discrepancy, because $k_1$ and $\omega$ are (for a given unit cell) the only input parameters to (C.1). Instead, the parity in magnitude between the terms featuring $\delta(\partial\phi_n/\partial\xi_1)$ and $\delta(\partial\phi_n/\partial\xi_2)$ – which preserves the sensitivity to $k_1$ – requires that

$$\left\|\delta\Big(\frac{\partial\phi_n}{\partial\xi_2}\Big)\right\|_{L^2_p(Y)} = O\left(\epsilon\left\|\delta\Big(\frac{\partial\phi_n}{\partial\xi_1}\Big)\right\|_{L^2_p(Y)}\right) = O\big(\epsilon\|\delta\nabla\phi_n\|_{L^2_p(Y)}\big), \tag{C.14}$$

which yields

$$\|\boldsymbol{e}_2\cdot\nabla\phi_n\|_{L^2_p(Y)} = O\big(\epsilon\,\|\boldsymbol{e}_1\cdot\nabla\phi_n\|_{L^2_p(Y)}\big) = O\big(\epsilon\,\|\nabla\phi_n\|_{L^2_p(Y)}\big). \tag{C.15}$$

## Appendix C.2 Skew Bravais lattice, $d\in\{2,3\}$.

We next seek to generalize (C.10) for a generic orthogonal Bravais lattice $\boldsymbol{R}\subset\mathbb{R}^d$, generic (rational) cut plane $\mathcal{S}$, and a generic (rational) direction of propagation $\boldsymbol{e}\parallel\mathcal{S}$.

**Proof of eq. (49).**

*Proof.* Recalling (7), a compact way to analyze QEP (15) in $\mathbb{R}^d$ with $\psi = \tilde{\phi}_n$ is to rewrite it using vector notation as

$$\int_{\tilde{Y}} G\,\nabla_{\tilde{\boldsymbol{k}}}\tilde{\phi}_n\cdot\nabla_{-\tilde{\boldsymbol{k}}}\overline{\tilde{\phi}_n}\,\mathrm{d}\tilde{Y}_{\tilde{\boldsymbol{x}}} - \omega^2\int_{\tilde{Y}}\rho\,\tilde{\phi}_n\,\overline{\tilde{\phi}_n}\,\mathrm{d}\tilde{Y}_{\tilde{\boldsymbol{x}}} = 0 \qquad \forall\psi\in H^1_p(\tilde{Y}), \tag{C.16}$$

where $\nabla_{\tilde{\boldsymbol{k}}} = \nabla + \mathrm{i}\tilde{\boldsymbol{k}}$ and

$$\begin{aligned}\nabla &= \frac{\partial}{\partial\tilde{x}^j}\tilde{\boldsymbol{b}}^j = \sum_\beta\frac{\partial}{\partial\tilde{x}^\beta}\tilde{\boldsymbol{b}}^\beta + \frac{\partial}{\partial\tilde{x}^\alpha}\tilde{\boldsymbol{b}}^\alpha,\\ \tilde{\boldsymbol{k}} &= \tilde{k}_j\,\tilde{\boldsymbol{b}}^j = \sum_\beta\tilde{k}_\beta\,\tilde{\boldsymbol{b}}^\beta + \tilde{\kappa}_n\,\tilde{\boldsymbol{b}}^\alpha,\end{aligned} \tag{C.17}$$

with implicit summation being assumed over the repeated index $j=\overline{1,d}$. For future reference, it is useful to note from the first of (C.17) that

$$\|\nabla\tilde{\phi}_n\|^2 = \left(\frac{\partial\tilde{\phi}_n}{\partial\tilde{x}^1},\dots,\frac{\partial\tilde{\phi}_n}{\partial\tilde{x}^d}\right)\cdot\tilde{\boldsymbol{\Gamma}}\cdot\overline{\left(\frac{\partial\tilde{\phi}_n}{\partial\tilde{x}^1},\dots,\frac{\partial\tilde{\phi}_n}{\partial\tilde{x}^d}\right)} \geqslant \tilde{\lambda}_{\min}\sum_{j=1}^d\left|\frac{\partial\tilde{\phi}_n}{\partial\tilde{x}^j}\right|^2, \tag{C.18}$$

locally, where $\tilde{\lambda}_{\min}$ is the smallest eigenvalue of the (symmetric, positive-definite) contravariant metric tensor $\tilde{\boldsymbol{\Gamma}}$ with components $\tilde{\Gamma}^{ij} = \boldsymbol{b}^i\cdot\boldsymbol{b}^j$. On recalling that $\{\tilde{k}_\beta\} = \{k_e, 0\}$, we conveniently introduce the scaling parameter

$$\epsilon = \epsilon(n) := \frac{|k_e|}{|\tilde{\kappa}_n|} = o(1) \tag{C.19}$$

and rescale the wave vector as

$$\tilde{\boldsymbol{k}} \;=\; \tilde{\kappa}_n \tilde{\boldsymbol{v}}, \qquad \tilde{\boldsymbol{v}} \;:=\; \epsilon\, e^{\mathrm{i}\varphi_n} \sum_{\beta} \delta_{\beta e} \tilde{\boldsymbol{b}}^{\beta} + \tilde{\boldsymbol{b}}^{\alpha}, \qquad \varphi_n \;=\; \arg\left(\frac{k_e}{\tilde{\kappa}_n}\right), \tag{C.20}$$

letting $\delta_{\beta e} = 1$ (resp. $\delta_{\beta e} = 0$) for the in-plane direction where $\tilde{k}_\beta = k_e$ (resp. $\tilde{k}_\beta = 0$). With such definition, (C.16) can be rewritten as

$$-\tilde{\kappa}_n^2 \tilde{\boldsymbol{v}}\cdot\tilde{\boldsymbol{v}} \int_{\tilde{Y}} G \tilde{\phi}_n \overline{\tilde{\phi}_n}\, \mathrm{d}\tilde{Y}_{\tilde{\boldsymbol{x}}} \;=\; 2\tilde{\kappa}_n \int_{\tilde{Y}} G \tilde{\boldsymbol{v}}\cdot\Im\left[\nabla\tilde{\phi}_n \overline{\tilde{\phi}_n}\right] \mathrm{d}\tilde{Y}_{\tilde{\boldsymbol{x}}} + \int_{\tilde{Y}} G \nabla\tilde{\phi}_n \cdot \nabla\overline{\tilde{\phi}_n}\, \mathrm{d}\tilde{Y}_{\tilde{\boldsymbol{x}}} - \omega^2 \int_{\tilde{Y}} \rho\, \tilde{\phi}_n \overline{\tilde{\phi}_n}\, \mathrm{d}\tilde{Y}_{\tilde{\boldsymbol{x}}}, \tag{C.21}$$

which yields

$$2|\tilde{\kappa}_n| \left| \int_{\tilde{Y}} G \tilde{\boldsymbol{v}}\cdot\Im\left[\nabla\tilde{\phi}_n \overline{\tilde{\phi}_n}\right] \mathrm{d}\tilde{Y}_{\tilde{\boldsymbol{x}}} \right| + \left| \int_{\tilde{Y}} G \nabla\tilde{\phi}_n \cdot \nabla\overline{\tilde{\phi}_n}\, \mathrm{d}\tilde{Y}_{\tilde{\boldsymbol{x}}} \right| + \omega^2 \rho_{\sup} \;\geqslant\; |\tilde{\kappa}_n|^2\, |\tilde{\boldsymbol{v}}\cdot\tilde{\boldsymbol{v}}|\, G_{\inf}. \tag{C.22}$$

Recalling that $\|\tilde{\phi}_n\|_{L^2_p(\tilde{Y})} = 1$, and letting

$$\tilde{\Gamma}^{\max} \;=\; \max_{i,j\in\overline{1,d}} \tilde{\Gamma}^{ij},$$

we find via repeated use of the triangle inequality and Cauchy-Schwarz inequality that

$$\begin{aligned}
\left| \int_{\tilde{Y}} G \tilde{\boldsymbol{v}}\cdot\Im\left[\nabla\tilde{\phi}_n \overline{\tilde{\phi}_n}\right] \mathrm{d}\tilde{Y}_{\tilde{\boldsymbol{x}}} \right| \;&\leqslant\; G_{\sup} \left| \int_{\tilde{Y}} \tilde{\boldsymbol{v}}\cdot\Im\left[\nabla\tilde{\phi}_n \overline{\tilde{\phi}_n}\right] \mathrm{d}\tilde{Y}_{\tilde{\boldsymbol{x}}} \right| \\
&\leqslant\; G_{\sup} \left\{ \epsilon \sum_{\beta} \delta_{\beta e} \sum_{j} |\tilde{\Gamma}^{\beta j}| \left| \int_{\tilde{Y}} \Im\left[\frac{\partial\tilde{\phi}_n}{\partial\tilde{x}^j} \overline{\tilde{\phi}_n}\right] \mathrm{d}\tilde{Y}_{\tilde{\boldsymbol{x}}} \right| + \sum_{j} |\tilde{\Gamma}^{\alpha j}| \left| \int_{\tilde{Y}} \Im\left[\frac{\partial\tilde{\phi}_n}{\partial\tilde{x}^j} \overline{\tilde{\phi}_n}\right] \mathrm{d}\tilde{Y}_{\tilde{\boldsymbol{x}}} \right| \right\} \\
&\leqslant\; G_{\sup} \tilde{\Gamma}^{\max} (1+\epsilon) \sum_{j} \left| \int_{\tilde{Y}} \Im\left[\frac{\partial\tilde{\phi}_n}{\partial\tilde{x}^j} \overline{\tilde{\phi}_n}\right] \mathrm{d}\tilde{Y}_{\tilde{\boldsymbol{x}}} \right| \\
&\leqslant\; G_{\sup} \tilde{\Gamma}^{\max} (1+\epsilon) \sum_{j} \left| \int_{\tilde{Y}} \left|\frac{\partial\tilde{\phi}_n}{\partial\tilde{x}^j} \overline{\tilde{\phi}_n}\right| \mathrm{d}\tilde{Y}_{\tilde{\boldsymbol{x}}} \right| \\
&\leqslant\; G_{\sup} \tilde{\Gamma}^{\max} (1+\epsilon) \sum_{j} \left\| \frac{\partial\tilde{\phi}_n}{\partial\tilde{x}^j} \right\|_{L^2_p(\tilde{Y})} \\
&\leqslant\; \sqrt{d}\, G_{\sup} \tilde{\Gamma}^{\max} (1+\epsilon) \left[ \sum_{j} \left\| \frac{\partial\tilde{\phi}_n}{\partial\tilde{x}^j} \right\|^2_{L^2_p(\tilde{Y})} \right]^{\frac{1}{2}} \\
&<\; 2\sqrt{d}\, G_{\sup} \tilde{\Gamma}^{\max} \left[ \sum_{j} \left\| \frac{\partial\tilde{\phi}_n}{\partial\tilde{x}^j} \right\|^2_{L^2_p(\tilde{Y})} \right]^{\frac{1}{2}}
\end{aligned} \tag{C.23}$$

for $\epsilon < 1$. Thanks to (C.18), we similarly find that

$$\left| \int_{\tilde{Y}} G \nabla\tilde{\phi}_n \cdot \nabla\overline{\tilde{\phi}_n}\, \mathrm{d}\tilde{Y}_{\tilde{\boldsymbol{x}}} \right| \;\leqslant\; G_{\sup} \left| \int_{\tilde{Y}} \|\nabla\tilde{\phi}_n\|^2\, \mathrm{d}\tilde{Y}_{\tilde{\boldsymbol{x}}} \right| \;\leqslant\; G_{\sup} \tilde{\Gamma}^{\max} \sum_{j=1} \left\| \frac{\partial\tilde{\phi}_n}{\partial\tilde{x}^j} \right\|^2_{L^2_p(\tilde{Y})}, \tag{C.24}$$

while

$$|\tilde{\boldsymbol{v}}\cdot\tilde{\boldsymbol{v}}| \;=\; \tilde{\Gamma}^{\alpha\alpha} \left| 1 + 2\epsilon e^{\mathrm{i}\varphi_n} \left\{ (\tilde{\Gamma}^{\alpha\alpha})^{-1} \sum_{\beta} \tilde{\Gamma}^{\beta\alpha} \right\} + (\epsilon e^{2\mathrm{i}\varphi_n})^2 \left\{ (\tilde{\Gamma}^{\alpha\alpha})^{-1} \sum_{\beta} \sum_{\gamma} \tilde{\Gamma}^{\beta\gamma} \right\} \right| \;>\; c' \tilde{\Gamma}^{\alpha\alpha} \tag{C.25}$$

for some $0 < c' < 1$ close to unity and sufficiently small $\epsilon$. Letting

$$\boldsymbol{g}_n \;:=\; \left(\frac{\partial\tilde{\phi}_n}{\partial\tilde{x}^1},\ldots,\frac{\partial\tilde{\phi}_n}{\partial\tilde{x}^d}\right)$$

and

$$\alpha \;:=\; \epsilon\,\|\boldsymbol{g}_n\|_{L^2_p(\tilde{Y})} \tag{C.26}$$

and substituting (C.23)–(C.25) into (C.22), we obtain

$$\alpha^2 + 4\sqrt{d}|k_e|\,\alpha \;>\; \gamma\,|k_e|^2, \qquad \gamma \;=\; c'\,\frac{G_{\inf}\tilde{\Gamma}^{\alpha\alpha}}{G_{\sup}\,\tilde{\Gamma}^{\max}} - \epsilon^2\,\frac{\omega^2\rho_{\sup}}{G_{\sup}\,\tilde{\Gamma}^{\max}} \;>\; c''\,\frac{G_{\inf}\tilde{\Gamma}^{\alpha\alpha}}{G_{\sup}\,\tilde{\Gamma}^{\max}} \tag{C.27}$$

and consequently

$$\alpha \;>\; |k_e|\left(\sqrt{4d+\gamma} - 2\sqrt{d}\right) \;>\; 0, \tag{C.28}$$

for sufficiently small $\epsilon$ and some $0 < c'' < c'$ (close to $c'$) that is independent of $\epsilon$. By virtue of (C.26) and (C.28), we obtain the lower bound

$$\|\boldsymbol{g}_n\|_{L^2_p(\tilde{Y})} \;>\; c\,|\tilde{\kappa}_n|, \qquad 0 \;<\; c \;\simeq\; \left(4d + \frac{G_{\inf}\tilde{\Gamma}^{\alpha\alpha}}{G_{\sup}\,\tilde{\Gamma}^{\max}}\right)^{\frac{1}{2}} - 2\sqrt{d}. \tag{C.29}$$

for sufficiently small $\epsilon$ i.e. large $|\tilde{\kappa}_n|$. The proof is completed by recalling (C.18) which, together with (C.29), yields the lower bound on the eigenfunction gradient as

$$\|\nabla\tilde{\phi}_n\|_{L^2_p(\tilde{Y})} \;\geqslant\; \lambda_{\min}^{1/2}\,\|\boldsymbol{g}_n\|_{L^2_p(\tilde{Y})} \;>\; \lambda_{\min}^{1/2}\,c\,|\tilde{\kappa}_n|. \tag{C.30}$$

□

### Justification of eq. (50).

Following the argument carried for an orthogonal lattice with $d = 2$, we find via perturbation analysis of (15) that the sensitivity of quadratic eigenmode variations to $k_e$ is, for large $|\tilde{\kappa}_n|$, preserved by the scaling of partials $(\partial\tilde{\phi}_n/\partial\tilde{x}^j)$ that balances the cross term

$$-\mathrm{i}\tilde{\kappa}_n\tilde{\Gamma}^{\alpha j}\int_{\tilde{Y}} G\left(\frac{\partial\tilde{\phi}_n}{\partial\tilde{x}^j}\overline{\psi} - \tilde{\phi}_n\frac{\partial\overline{\psi}}{\partial\tilde{x}^j}\right)\mathrm{d}\tilde{Y}_{\tilde{\boldsymbol{x}}} \;-\; \mathrm{i}\sum_\beta \tilde{k}_\beta\tilde{\Gamma}^{\beta j}\int_{\tilde{Y}} G\left(\frac{\partial\tilde{\phi}_n}{\partial\tilde{x}^j}\overline{\psi} - \tilde{\phi}_n\frac{\partial\overline{\psi}}{\partial\tilde{x}^j}\right)\mathrm{d}\tilde{Y}_{\tilde{\boldsymbol{x}}} \tag{C.31}$$

in (15) for all $\psi \in H^1_p(\tilde{Y})$, where $j = \overline{1,d}$, $\beta = \overline{1,d}\backslash\{\alpha\}$, and implicit summation is assumed over the repeated index $j$. Recalling the second of (C.17), we specifically note that

$$\begin{aligned}\tilde{\boldsymbol{k}}\cdot\nabla\tilde{\phi}_n \;&=\; \tilde{\kappa}_n\,\tilde{\boldsymbol{b}}^\alpha\cdot\nabla\tilde{\phi}_n \;+\; \sum_\beta \tilde{k}_\beta\,\tilde{\boldsymbol{b}}^\beta\cdot\nabla\tilde{\phi}_n \\ &=\; \tilde{\kappa}_n\,\tilde{\Gamma}^{\alpha j}\,\frac{\partial\tilde{\phi}_n}{\partial\tilde{x}^j} \;+\; \sum_\beta \tilde{k}_\beta\,\tilde{\Gamma}^{\beta j}\,\frac{\partial\tilde{\phi}_n}{\partial\tilde{x}^j}.\end{aligned} \tag{C.32}$$

By requiring the parity (in order of magnitude) between the two summands in (C.31), from (C.32) we obtain the scaling relationship

$$\|\tilde{\boldsymbol{b}}^\alpha\cdot\nabla\tilde{\phi}_n\|_{L^2_p(\tilde{Y})} \;=\; O\big(\epsilon\,\|\tilde{\boldsymbol{b}}^\beta\cdot\nabla\tilde{\phi}_n\|_{L^2_p(\tilde{Y})}\big) \qquad \text{for } \beta = \{\overline{1,d}\}\backslash\{\alpha\} \quad \text{s.th.} \quad \tilde{\boldsymbol{b}}^\beta \parallel \boldsymbol{e}, \tag{C.33}$$

noting that the $\beta$-qualifier caters for $d = 3$ where $\{\tilde{k}_\beta\} = \{k_e, 0\}$. In the latter case, no information is (at this point) available on the variation of $\nabla\tilde{\phi}_n$ in the "other" in-plane direction, $\tilde{\boldsymbol{b}}^\beta$, for which $\tilde{k}_\beta = 0$.

# Appendix D Numerical evidence

## Appendix D.1 QEP eigenfunctions

In this section, we plot the first 25 QEP eigenfunctions over the unit cell $Y$ (resp. $\tilde{Y}$) for the 0:1 (resp. 1:2) rational cut made on a square lattice $\boldsymbol{R} \subset \mathbb{R}^2$ endowed with unit cell (65). As can be seen from Fig. D.1 and Fig. D.2, the featured distributions of $\phi(\boldsymbol{x})$ and $\tilde{\phi}(\boldsymbol{x})$ support the claims made in Section 33.4.

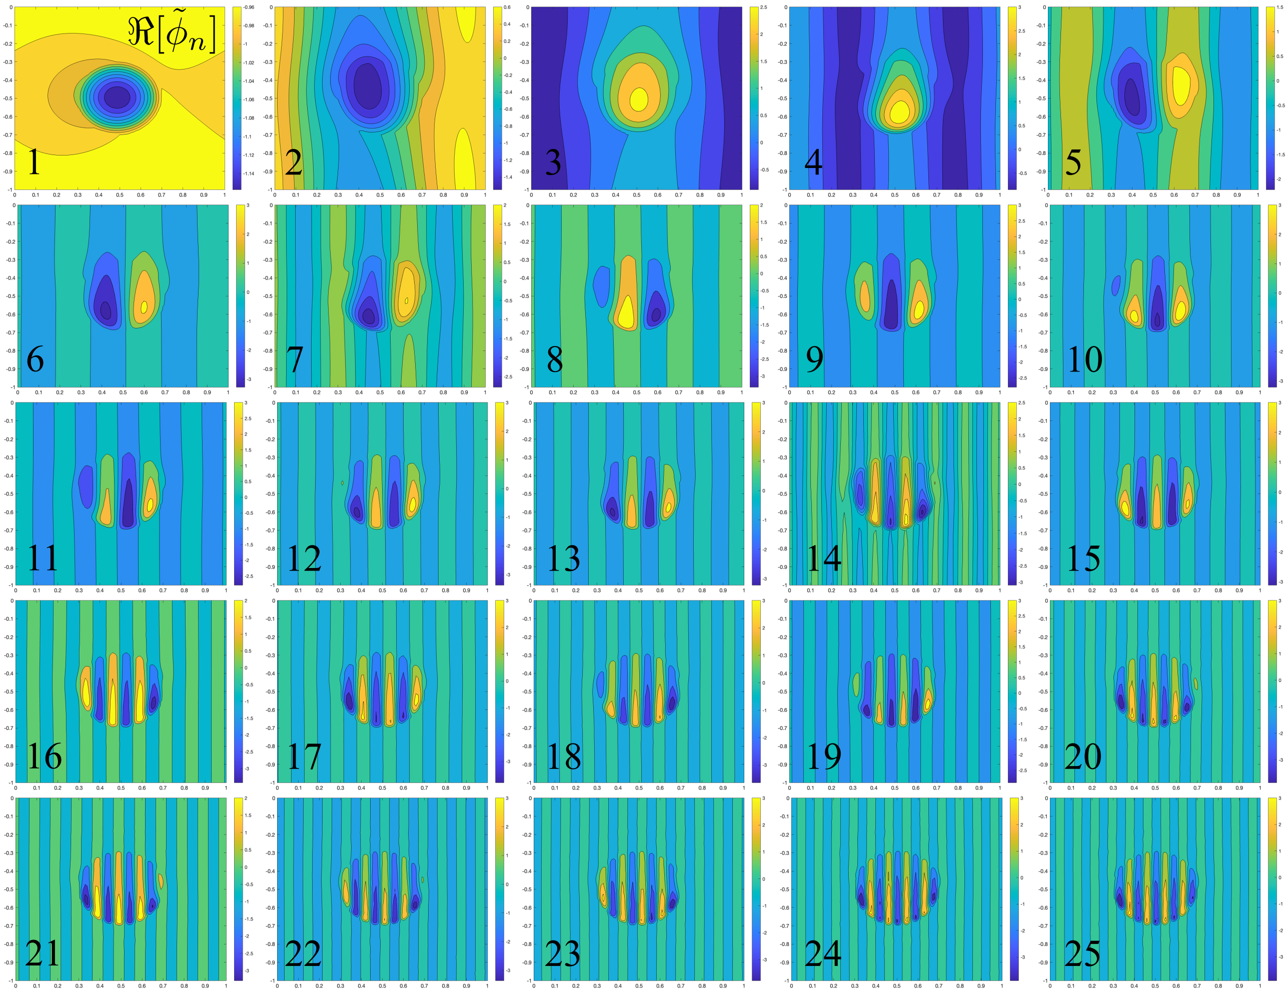


Figure D.1: Distribution of the eigenfunctions $\phi_n(\boldsymbol{x})$, $n = \overline{1,25}$ (real parts) solving QEP (9) over the unit cell $Y$ for a 0:1 horizontal cut ($q^1 = 1$, $q^2 = 0$) made on a square lattice $\boldsymbol{R} \subset \mathbb{R}^2$ endowed with the unit cell (65). The direction of propagation of the surface Bloch wave is $\boldsymbol{e} = \boldsymbol{e}_1$, where $(\boldsymbol{e}_1, \boldsymbol{e}_2)$ is the orthonormal basis aligned with the lattice basis vectors.

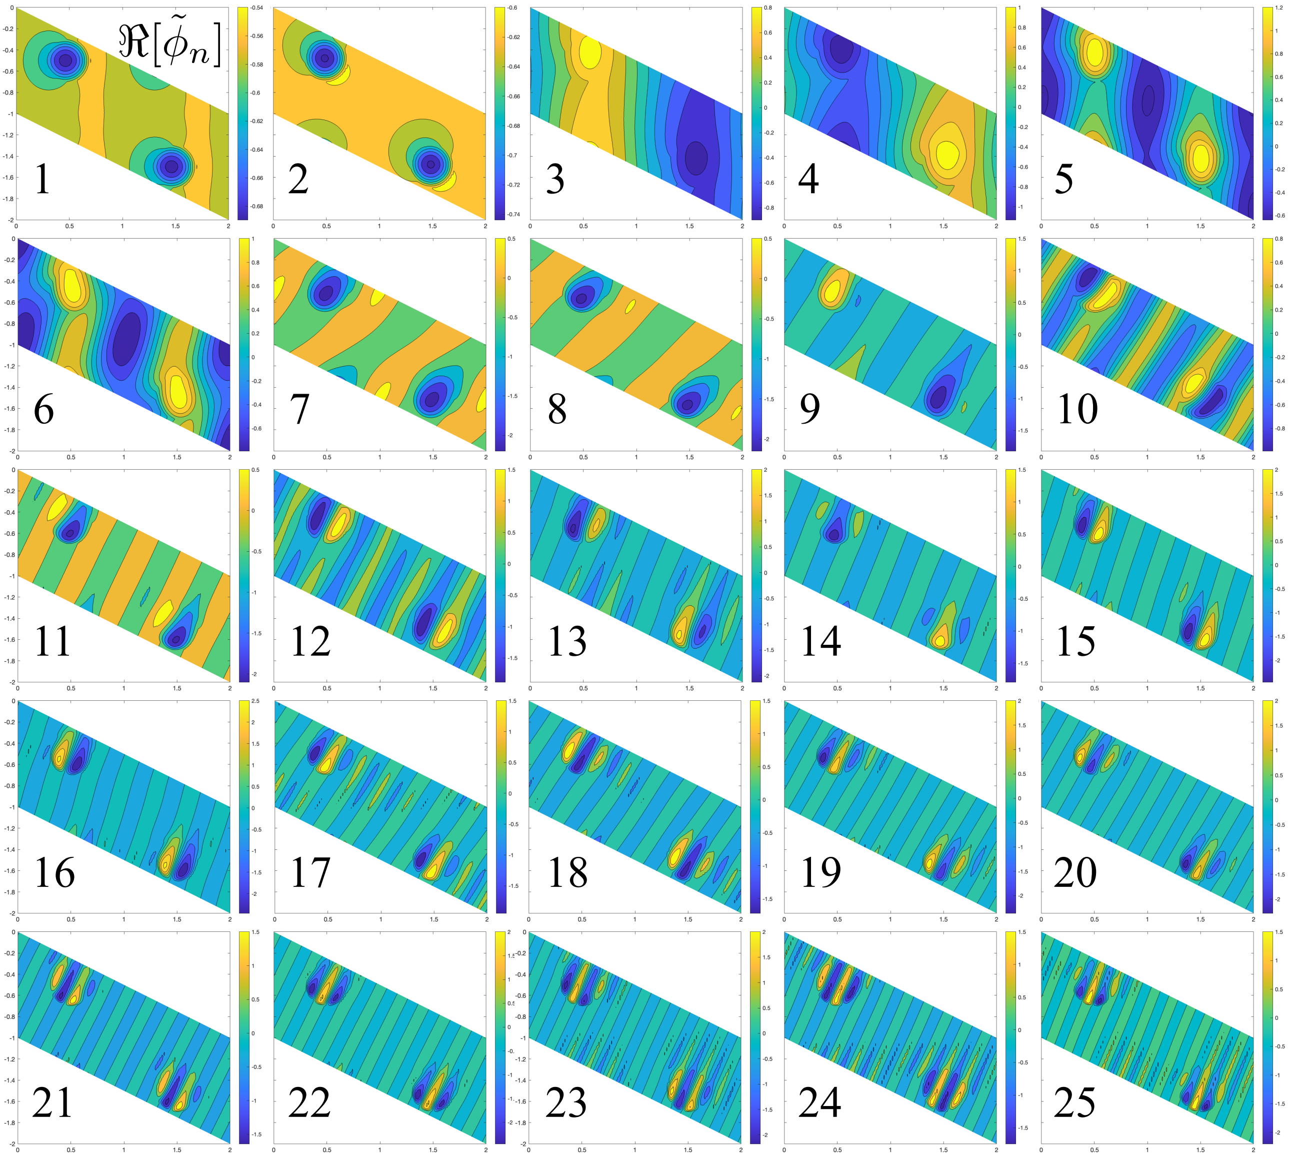

Figure D.2: Distribution of the eigenfunctions $\tilde{\phi}_n(\boldsymbol{x})$, $n = \overline{1, 25}$ (real parts) solving QEP (15) over the unit cell $\tilde{Y}$ for a 1:2 rational cut ($q^1 = 2$, $q^2 = 1$) made on a square lattice $\boldsymbol{R} \subset \mathbb{R}^2$ endowed with the unit cell (65). The direction of propagation of the surface Bloch wave is $\boldsymbol{e} = (2\boldsymbol{e}_1 + \boldsymbol{e}_2)/\sqrt{5}$, where $(\boldsymbol{e}_1, \boldsymbol{e}_2)$ is the orthonormal basis aligned with the lattice basis vectors.

## Appendix D.2 "Eiffel tower" diagrams

With reference to Fig. 5 in the manuscript and affiliated discussion in Section 55.1, Fig. D.3 plots the distributions of the condition number $C_{\boldsymbol{\Psi}}(k_e)$ at 14 frequencies inside the first pass band. As seen from the display, at each sampled frequency $C_{\boldsymbol{\Psi}}(k_e)$ features a pronounced peak that locates a point on the SB dispersion diagram (see Fig. 5). Here it is worth noting that the magnitude of each peak is limited by the resolution of wavenumber sampling, and can generally be increased by refining the sampling grid.

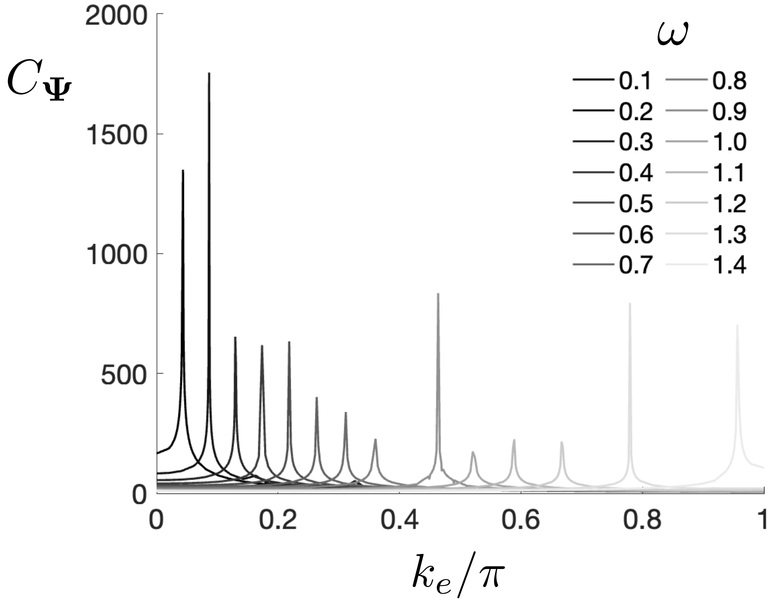


Figure D.3: Variations of the condition number $C_{\mathbf{\Psi}}(k_e)$ featured by the matrix $\mathbf{\Psi}(k_e)$ of the surface-wave eigenproblem (34) over the positive half of the Brillouin zone for $\omega = n/10$, $n = \overline{1,14}$. The results are computed for a square lattice with unit cell (65) and 0:1 horizontal cut made at depth $\mathfrak{d} = -0.5$. At each frequency $\omega$, location of the peak identifies the wavenumber $k_e = k_e^\star$ of the surface Bloch wave.
